# Supplementary material for: Applied Nanofabrication for X-ray Grating Spectroscopy
Source: arXiv:2103.10470 source file (2022-06-16)
Supplement: Supplementary file 5 [file Dedication.tex]

% Place the dedication below.
This dissertation is dedicated to my maternal great-grandmother, Edith Hatch Allen, my paternal grandfather, Richard Edward McCoy, and my maternal uncle, Jon Howard Hextell.
